# Supplementary material for: CLOAF: CoLlisiOn-Aware Human Flow
Source: arXiv:2403.09050 source file (2024-03-14)
Supplement: Supplementary file 1 [file supp_ablation_re.tex]

% !TEX root = ../top.tex
% !TEX spellcheck = en-US

\begin{figure}[t!]
 \centering
  \includegraphics[width=\linewidth]{supp/figs/supp_ablation_re.pdf}
   \caption{
       \small{{\bf Relative Error for various $\|\delta\Theta\|$.}
       It significantly drops around $S=100\div 1000$ sampled points, disregarding the value of $\|\delta\Theta\|$. 
}}
    \label{fig:ablation_re}
\end{figure}
